# Supplementary material for: Langevin equations for landmark image registration with uncertainty
Source: arXiv:1605.09276 source file (2017-01-06)
Supplement: Supplementary file 1 [file sde_imag_supplement.pdf]

# SUPPLEMENTARY MATERIALS: Langevin equations for landmark image registration with uncertainty *

Stephen Marsland† and Tony Shardlow‡

The examples and algorithms in the main article were generated with a set of Python codes available at https://github.com/tonyshardlow/reg_sde. Here, we provide further example sets generated by the code.

**SM1. Registration with known landmarks.** We show the performance and results of the solver for the Hamiltonian boundary-value problem. The solver uses an explicit Euler approximation with a single- or multiple-shooting method. Scipy's nonlinear equation solver `root` (with `hybr` and `lm` options) is used to solve the nonlinear system of equations. Consider a length scale `ell`, a Numpy array `LM` of landmarks (with `LM[i,j,k]` denoting the $i$th landmark set, for the $j$th dimension of the $k$th landmark), and a chosen number of time steps `no_steps` (single natural number for single shooting, a list of two numbers for multiple shooting indicating the number of steps per shoots and the number of shoots). Then, we may the solve the registration problem with

```
import hamiltonian
import diffeo
G=hamiltonian.GaussGreen(ell)
if isinstance(no_steps, list):
  ODE=diffeo.MultiShoot(G)
else:
  ODE=diffeo.Shoot(G)  # use single shooting
ODE.set_no_steps(no_steps)
ODE.set_landmarks(LM)
ODE.solve()
```

Landmark data can be centered to have mean zero and pre-registered with an orthogonal Procrustes transformation, via

```
import utility
LM=utility.procrust1(LM)
```

This is done for all the examples included in this paper.

The resulting registration (also known as a warp) can be plotted in Matplotlib with

```
import matplotlib as mpl
import pylab as plt
utility.plot_setup()
plt.axis('equal')
utility.plot_RT(LM)
ODE.plot_warp()
```

*This work was partially supported by the LMS Scheme 7 grant SC7-1415-09.
†Massey University s.r.marsland@massey.ac.nz
‡Department of Mathematical Sciences, University of Bath, Bath BA2 7AY, UK t.shardlow@bath.ac.uk



DRAFT

*This manuscript is for review purposes only.*

| $\delta^2$ | concentric | | $\delta^2$ | squashed | | wrap | | shark | |
|---|---|---|---|---|---|---|---|---|---|
| | single | multi | | single | multi | single | multi | single | multi |
| 0 | 0.1 | 0.3 | 0 | 0.1 | 0.3 | 267.5 | 1.3 | 2.5 | 0.8 |
| 0.01 | 0.2 | 0.4 | 0.001 | 0.2 | 0.3 | 4.7 | 2.4 | 0.4 | 0.8 |
| 0.015 | 0.3 | 0.6 | 0.0015 | 0.3 | 0.4 | 1.4 | 1.8 | 0.4 | 0.7 |
| 0.02 | 1.4 | 0.3 | 0.002 | 1.3 | 0.4 | 39 | 1.3 | 0.4 | 1.5 |

**Figure SM1.** *Execution time in seconds for experiments in Figures SM2 to SM5 for solving the boundary-value problem with shooting using twenty-five steps or with multiple-shooting using five shoots of five steps. The parameter $\delta^2$ is the variance of the noise added to each landmark in the data set.*

.

The warp is applied to an image (assuming $[-1,1]\times[-1,1]$ for the co-ordinate system) via

```
import skimage
from skimage import data
image = data.coffee() # load example image
new_image=ODE.warp(image)
```

and `imshow` can be used to view the image. See Figure SM6.

Four examples are shown with four levels of noise added to the landmarks in Figures SM2 to SM5. Here we use length scale $\ell = 0.5$ (for the Green's function). These can be generated with the script `run_supp_bvp.py`.

**Concentric** Figure SM2 shows twenty landmarks on two concentric circles of radii $r = 1, 2$ perturbed by mean-zero *iid* Gaussian noise with variances $0, 0.01, 0.015, 0.02$.

**Squashed** Figure SM3 shows a circle and squashed ellipse, with twenty landmarks each, perturbed by mean-zero *iid* Gaussian noise with variances $0, 0.001, 0.0015, 0.002$.

**Wrap** Figure SM4 shows an ellipse and a wrapped shape, with thirty landmarks each, with the same noise added as Figure SM3.

**Shark** Figure SM5 shows a shark and plane shape, with thirty landmarks each, with the same noise added as Figure SM3.

Detailed execution times on a 3.1Ghz 8GB PC using Python 2.7 are shown in Figure SM1. In general, single shooting is fast enough, but some bad configurations cause very significant slow down. Due to the potential for large momenta as part of the multiple-shooting solution, it is essential for the Python nonlinear solver to scale the momentum variables (by providing an array `'diag'`).

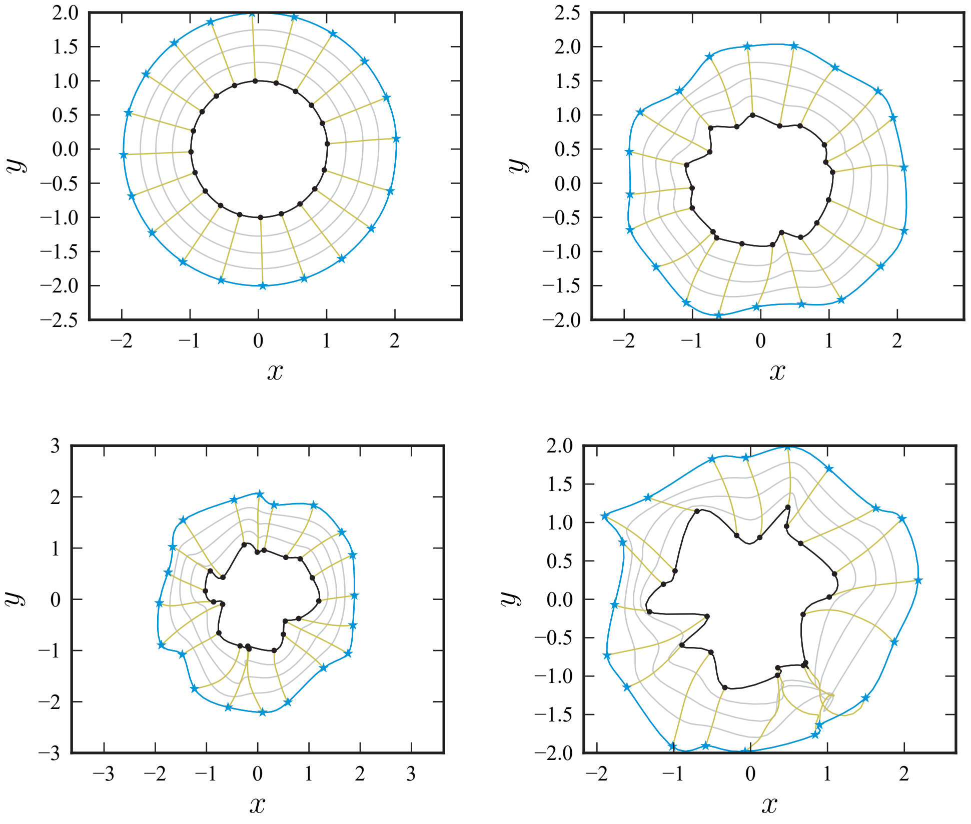


**Figure SM2.** *Classical registration by landmark matching for concentric circles. Here and in all other figures ⋆ marks the target landmarks.*

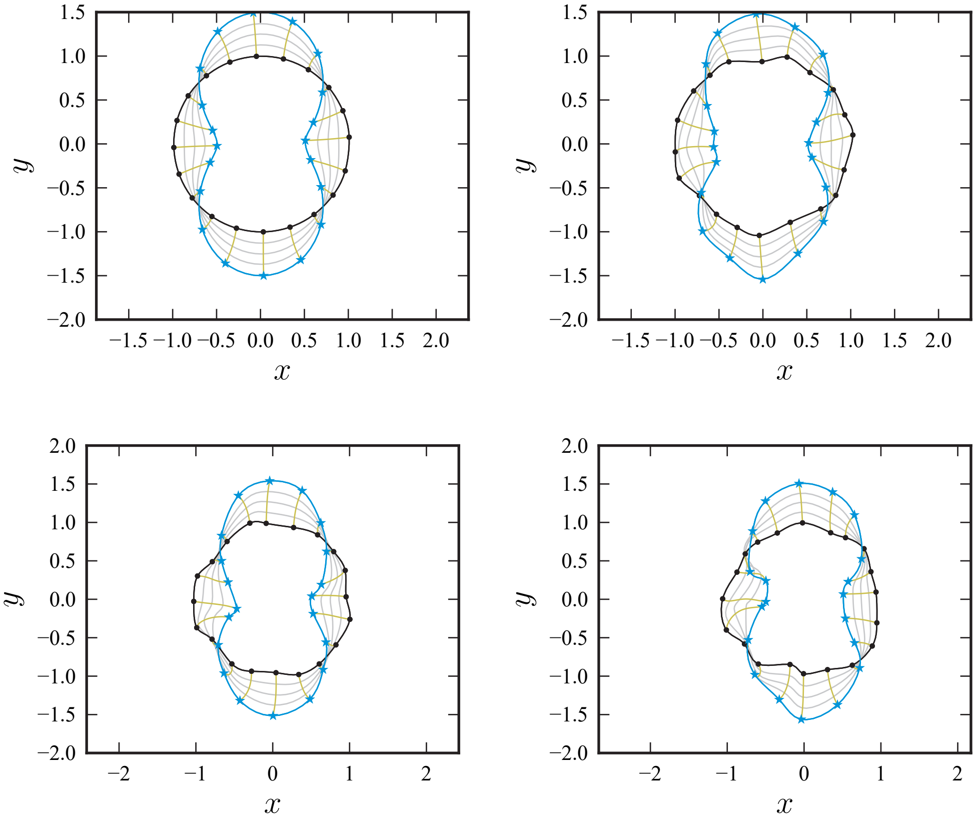


**Figure SM3.** *Classical registration by landmark matching for squashed ellipse.*

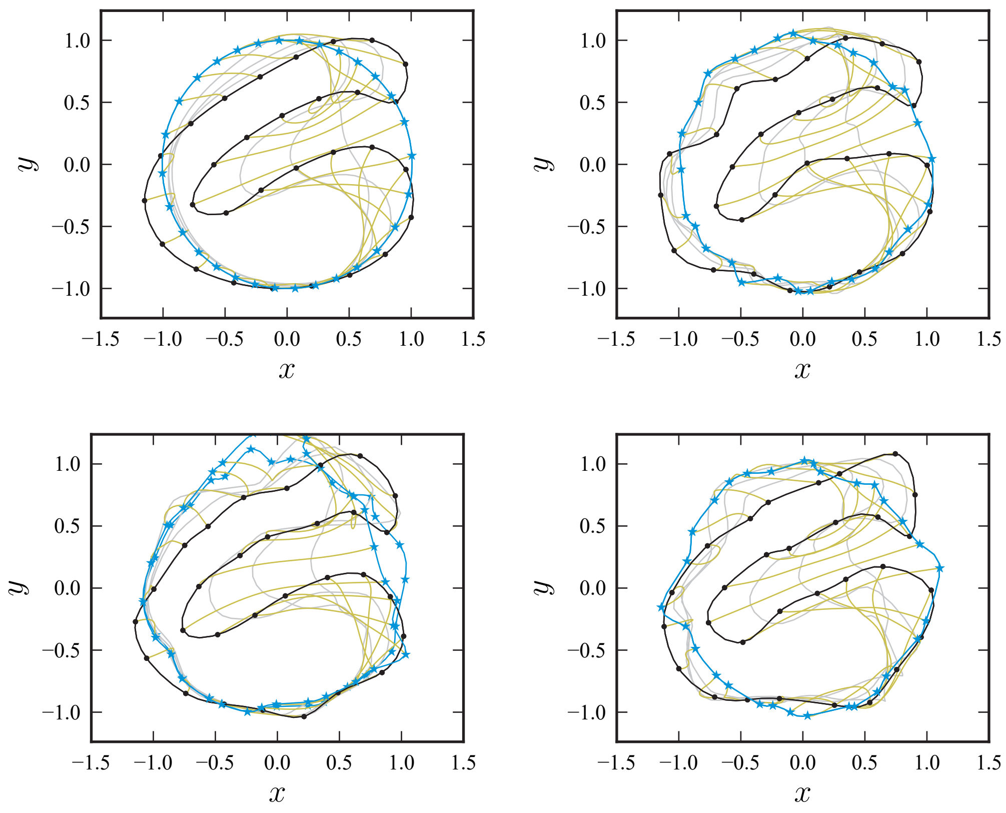


**Figure SM4.** *Classical registration by landmark matching for wrap.*

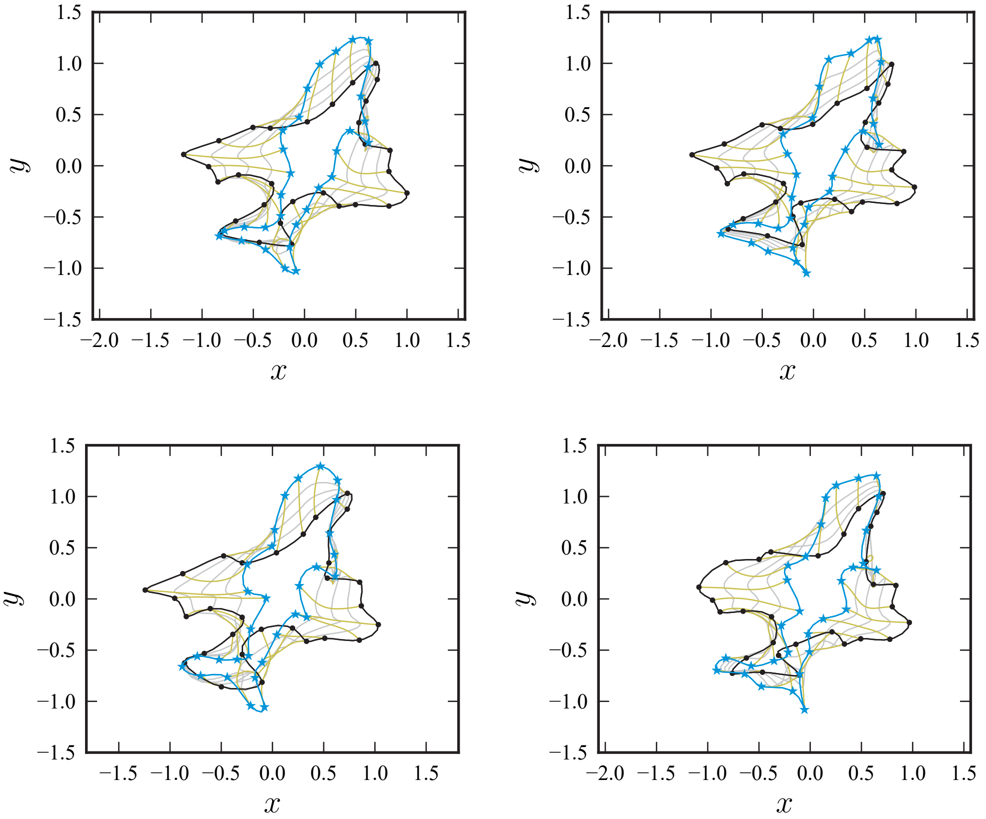


**Figure SM5.** *Classical registration by landmark matching for shark.*

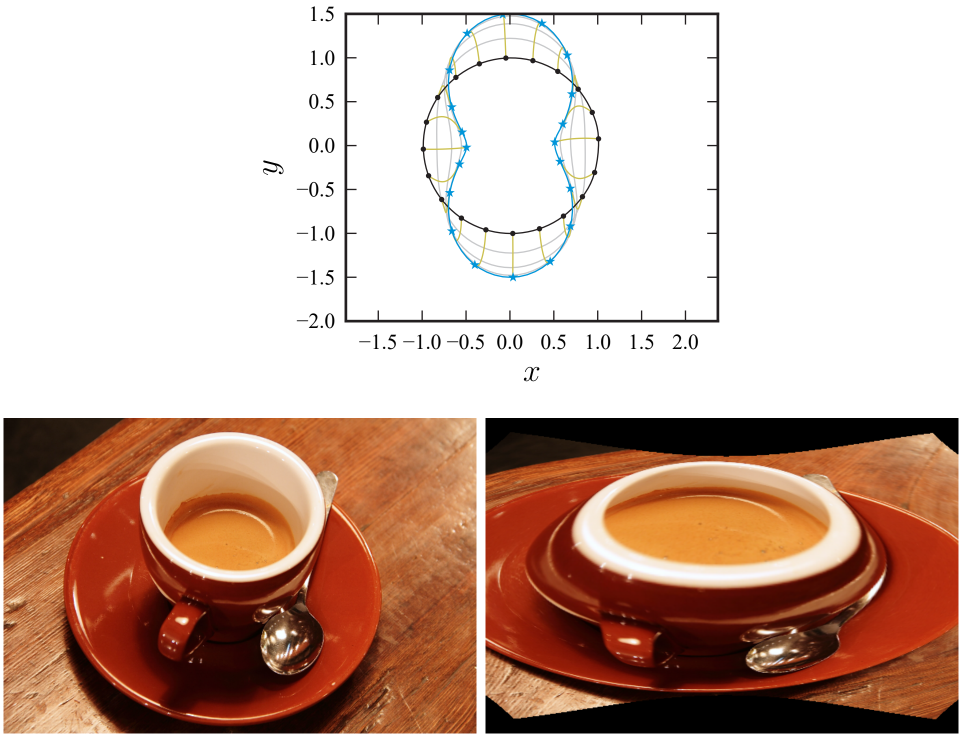


**Figure SM6.** *Classical registration by landmark matching, with example image.*

**SM2. Linearised-Langevin prior.** Given the `ODE` object created by Python above, we run the linearised-Langevin registration as follows. It requires `lam` and `beta` for $\lambda$ and $\beta$, the Langevin parameters, and `epsilon_prior` to define the initial prior distribution, and `data_var` for the data variance.

```
import sde
SDE = sde.SDELin(ODE)
SDE.set_lam_beta(lam,beta)
SDE.set_lin_path(ODE.Ppath,ODE.Qpath)
SDE.set_prior_eps(epsilon_prior)
SDE.do_all(data_var)
```

We always choose `epsilon_prior` equal to `data_var`, which is the variable $\delta^2$ indicated in the figure captions. Plotting of the registration can be achieved with

```
utility.plot_setup()
SDE.sd_plot()
```

Figures SM7 to SM10 show four examples. The whole example set can be reproduced via the `run_supp_lin.py` script.

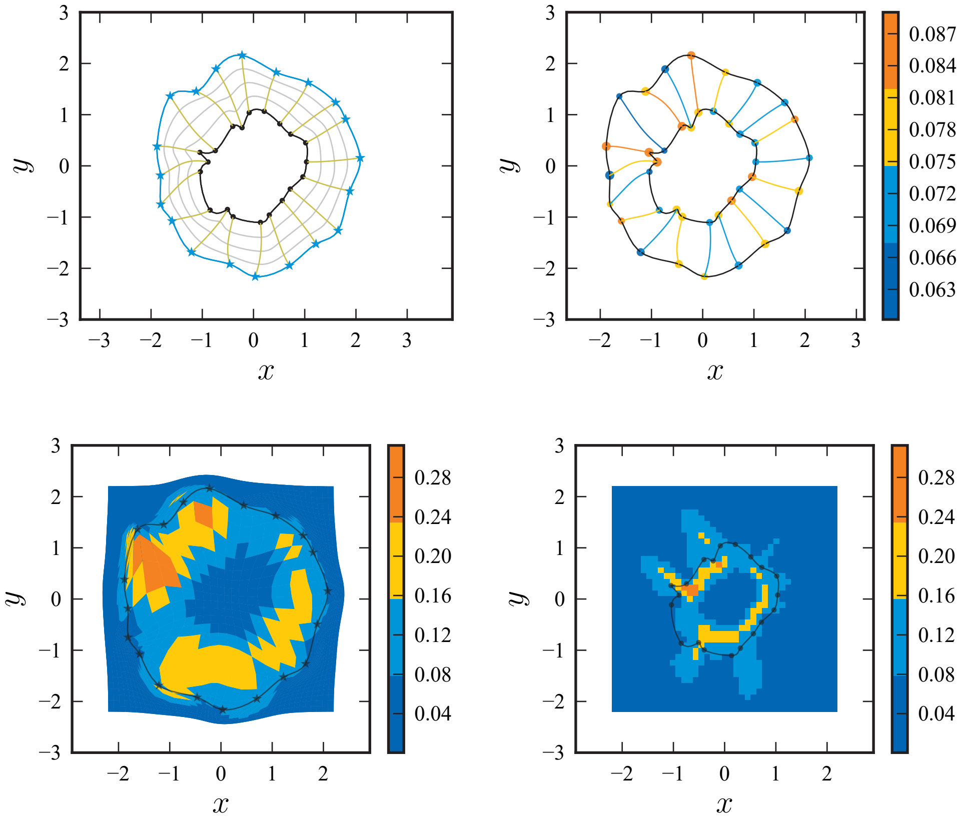


**Figure SM7.** *Using linearised-Langevin prior for concentric circles with* $\lambda = 0.01$*,* $\beta = 1000$*, and* $\delta^2 = 0.01$*. Colours mark standard deviations at the landmarks (top-right) and the diffeomorphism on a grid of points in the transformed co-ordinate system (bottom left) and original co-ordinate system (bottom right).*

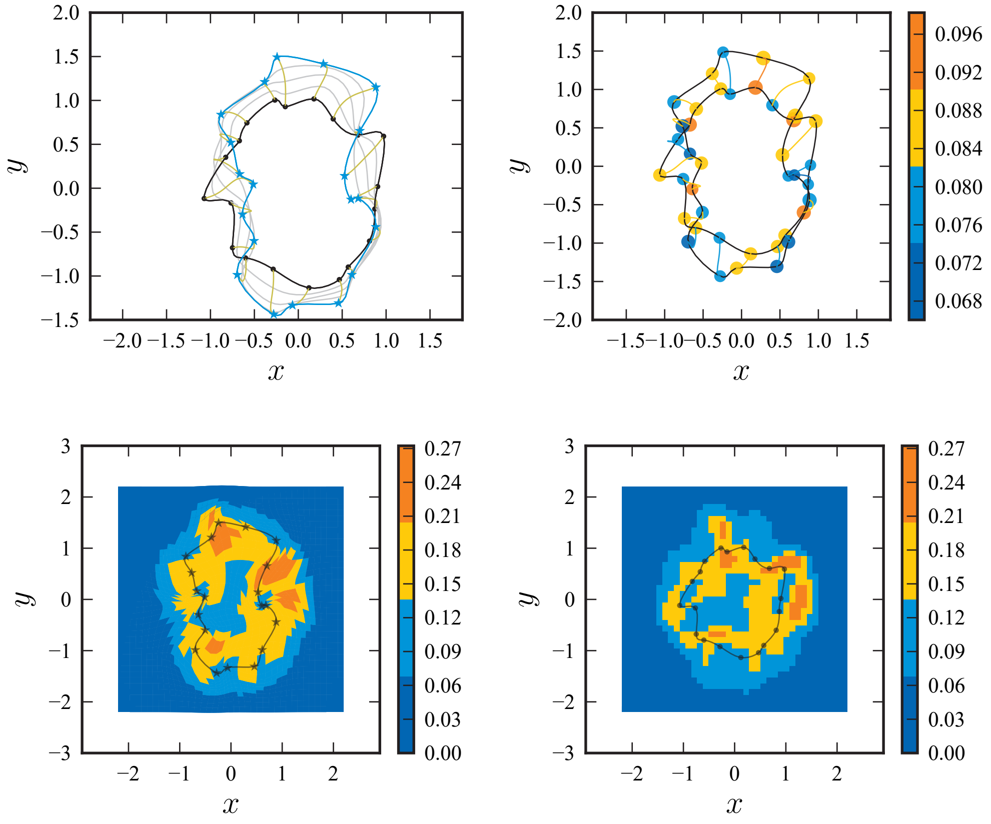


**Figure SM8.** *Linearised Langevin prior for squashed ellipse with* $\lambda = 0.1$ *and* $\beta = 100$ *and* $\delta^2 = 0.01$.

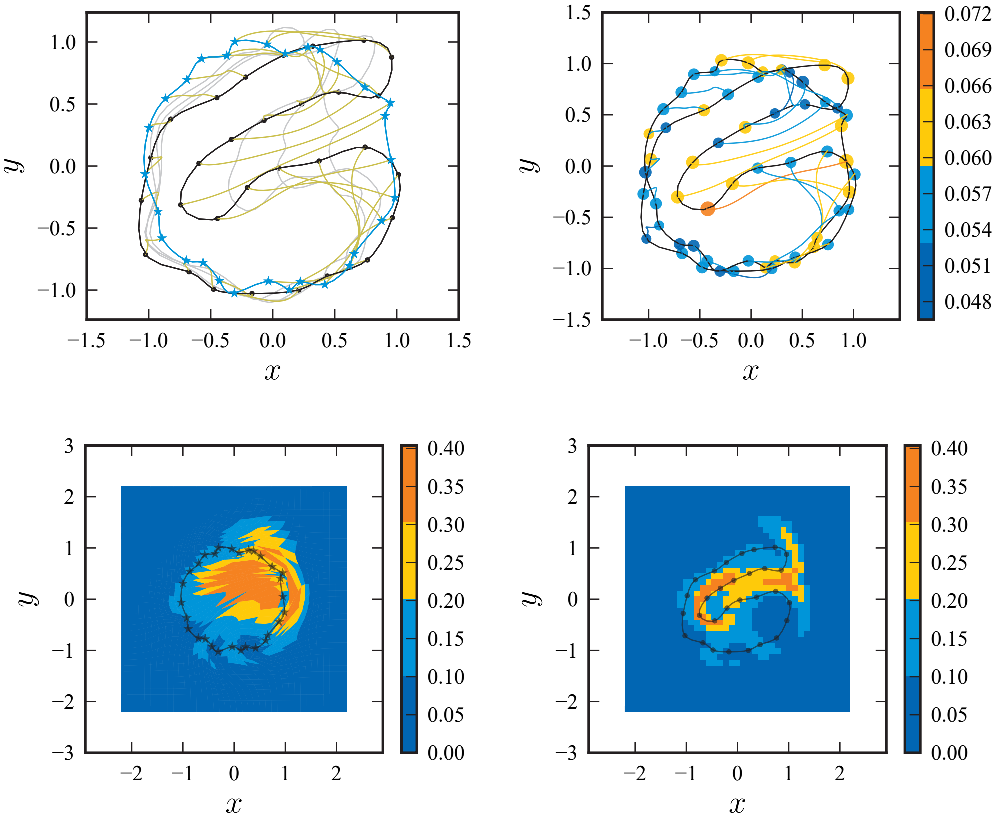


**Figure SM9.** *Registration using the linearised-Langevin prior for wrap for* $\lambda = 0.1$, $\beta = 1000$, *and* $\delta^2 = 0.05$.

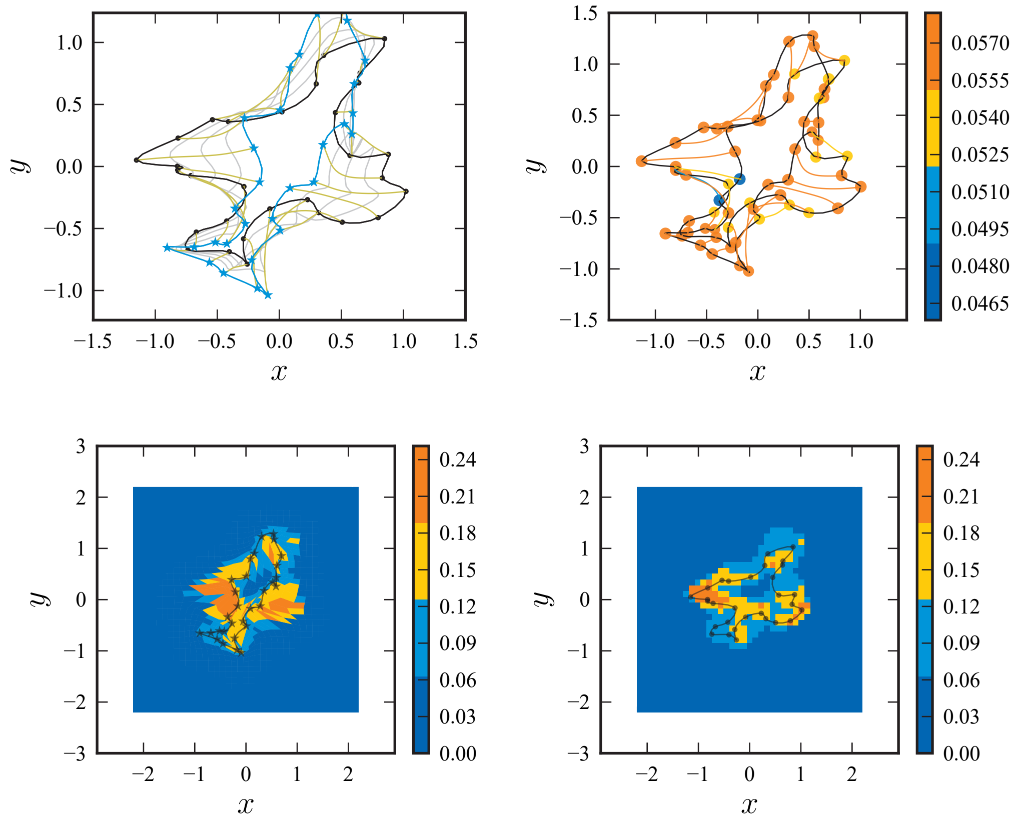


**Figure SM10.** *Registration using the linearised-Langevin prior for shark dataset with* $\lambda = 0.1$*,* $\beta = 0.5$*, and* $\delta^2 = 0.0025$*.*

| | concentric | squashed | wrap | shark |
|---|---|---|---|---|
| top row | 3 | 1 | 2 | 3.9 |
| bottom row | 3 | 1.7 | 2 | 4 |

**Figure SM11.** *Execution time in seconds for experiments with first splitting prior in Figures SM12 to SM15.*

.

**SM3. First splitting prior.** This experiment uses the first splitting prior with noisy observations to define a registration and uses a Laplace approximation of the posterior distribution to establish a standard deviation for the MAP reference landmarks. All experiments are based on twenty-five time steps. Columns are independent samples for the same problem. Rows show different inverse temperatures. In the bottom row, the $\beta$ is larger so that the data is neglected in favour of a lower bending energy. All landmarks are perturbed from an initial data set by mean-zero *iid* Gaussian noise with variance $\delta^2$. The length scale for the Green's function is unchanged from the corresponding experiment in §SM1.

```
SDE=sde.MAP1(G)
SDE.set_no_steps(no_steps)
SDE.set_landmarks(LM)
SDE.set_data_var(data_var)
SDE.set_lam_beta(lam, beta) # lam is not used by MAP1
SDE.solve()
```

To plot the results,

```
utility.plot_setup()
SDE.plot_warp()
cov_q,cov_p=SDE.cov()
utility.add_sd_plot(SDE.Qrn, cov_q)
```

Four examples are shown in Figures SM12 to SM15. The whole example set can be reproduced via the `run_supp_split1.py` script.

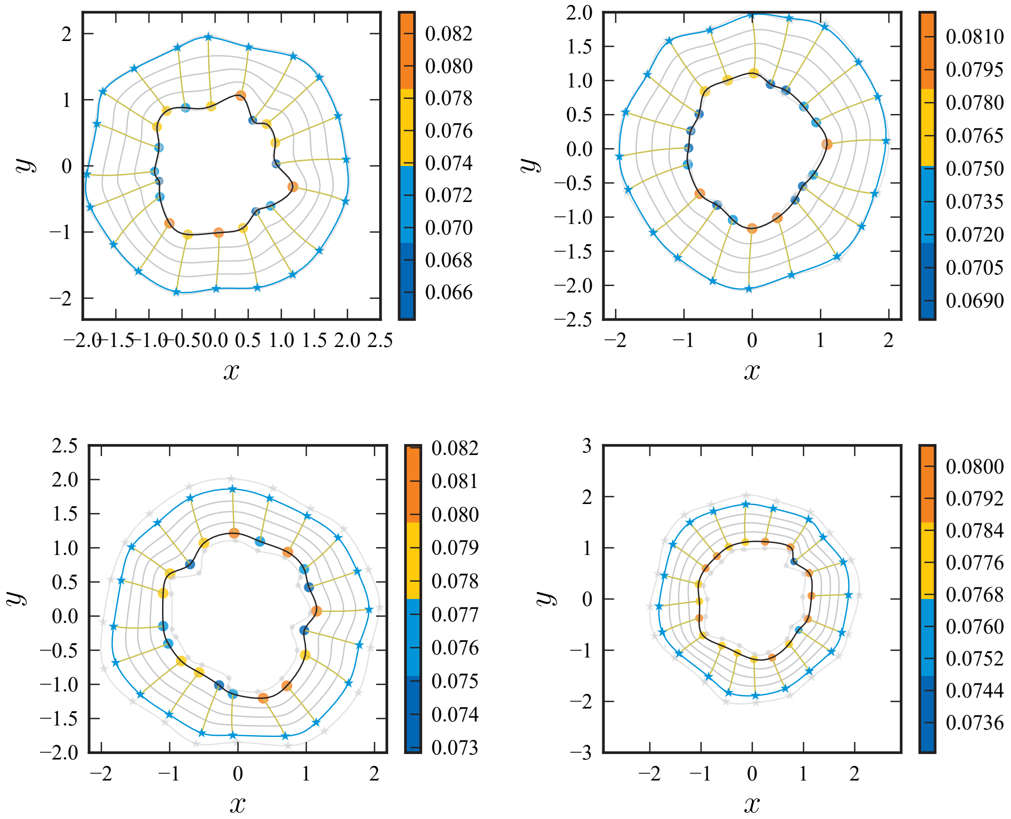


**Figure SM12.** *First splitting prior for concentric circles: the discs on the reference landmarks indicate one standard deviation of the computed posterior covariance. Top row: two examples with* $\beta = 4$*; bottom row: two examples with* $\beta = 40$*. In all examples, the data variance is* $\delta^2 = 0.005$ *(so* $\delta \approx 0.07$*)*

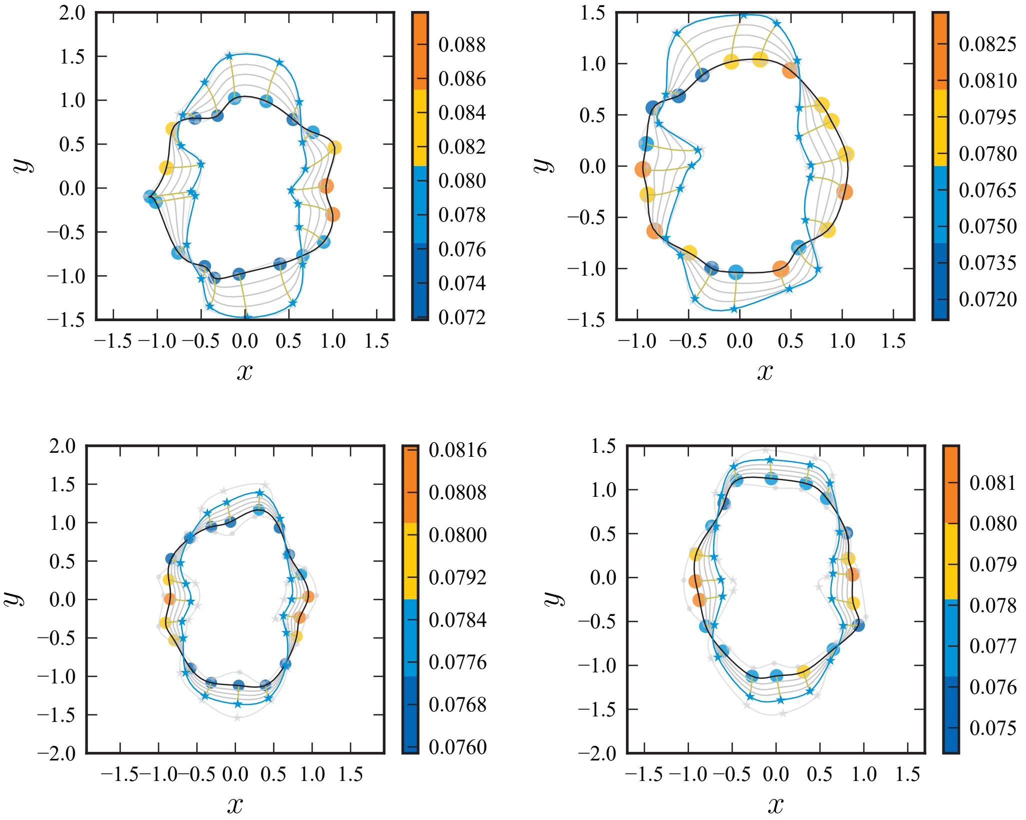

**Figure SM13.** *First splitting prior for the squashed ellipse. Top row:* $\beta = 4$*, bottom row* $\beta = 100$*. All* $\delta^2 = 0.005$ *(so* $\delta \approx 0.07$*)*

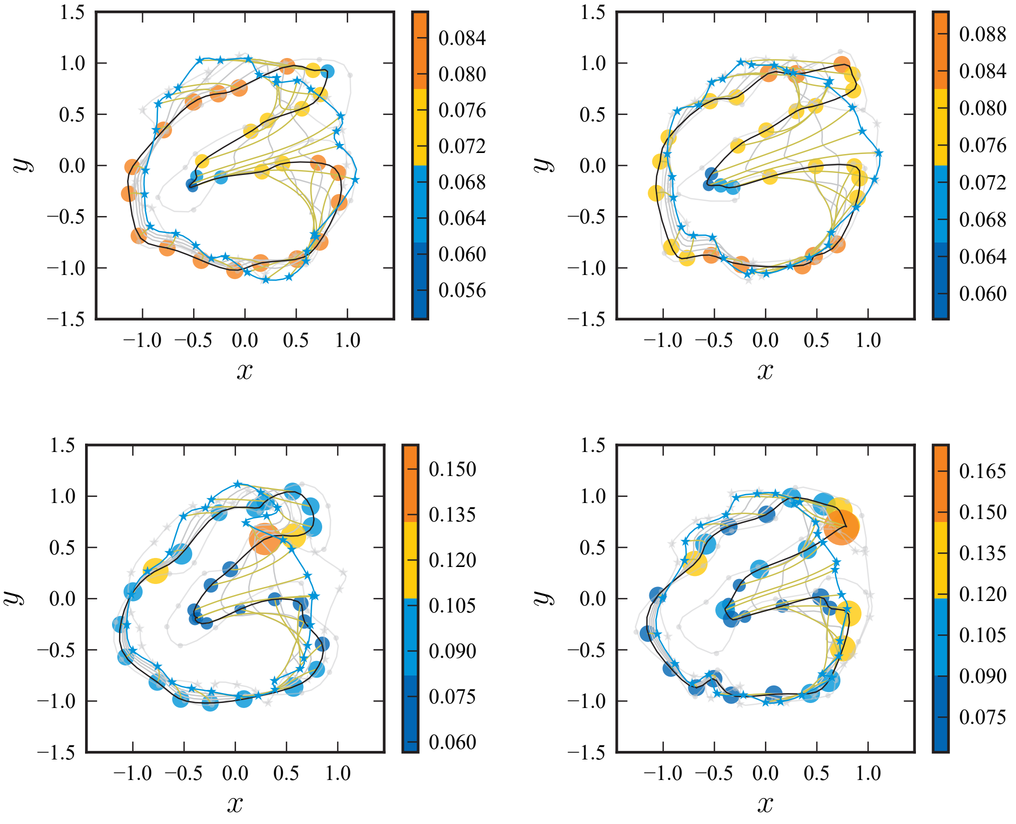


**Figure SM14.** *First splitting prior for the wrap. Top row: $\beta = 8$, bottom row $\beta = 100$. All $\delta^2 = 0.005$ (so $\delta \approx 0.07$)*

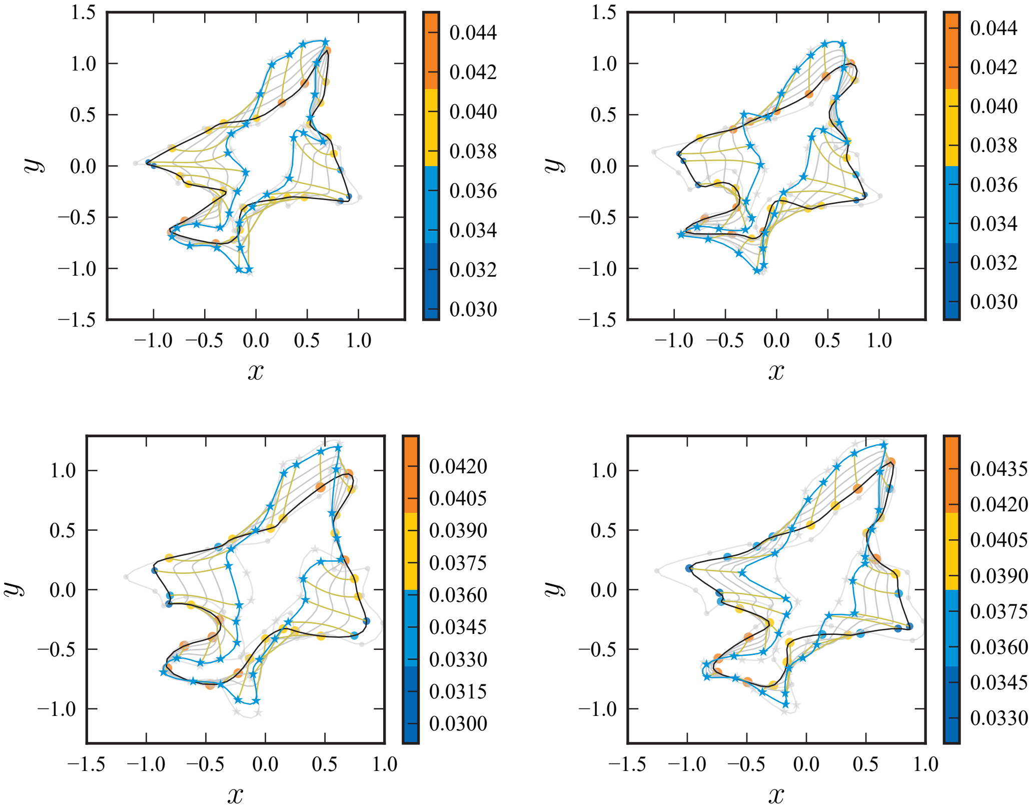


**Figure SM15.** *First splitting prior for the shark. The top row shows two examples with* $\beta = 0.5$*, and the bottom row shows two examples with* $\beta = 100$*. In all cases,* $\delta^2 = 0.00125$ *(so* $\delta \approx 0.035$*)*

| samples | concentric | squashed | wrap | shark |
|---|---|---|---|---|
| 2 | 1.4 | 1.2 | 3.8 | 2.9 |
| 10 | 3.3 | 1.8 | 3.5 | 6.7 |

**Figure SM16.** *Execution time in seconds for experiments with second splitting prior in Figures SM17 to SM20.*

.

## SM4. Second splitting prior.

In Figures SM17 to SM20, we show experiments with the second splitting prior and computations of the average of sets of landmarks. The left-hand column shows two (top) and ten (bottom) landmark sets, with the computed average landmarks shown in the right-hand column. The arithmetic average is given along with the MAP point for the second splitting prior (the discs mark one standard deviation of the computed posterior covariance).

The following calls are used:

```
SDE=sde.MAP4(G)
SDE.set_data_var(data_var)
SDE.set_lam_beta(lam,beta)
SDE.set_landmarks(LM)
SDE.set_no_steps(no_steps)
SDE.solve()
cov_q,cov_p=SDE.cov()
```

To plot the results,

```
utility.plot_setup()
utility.plot_average(SDE.Qh)
utility.add_sd_plot(SDE.Qh, cov_q)
```

The whole example set can be reproduced via the `run_supp_split2.py` script.

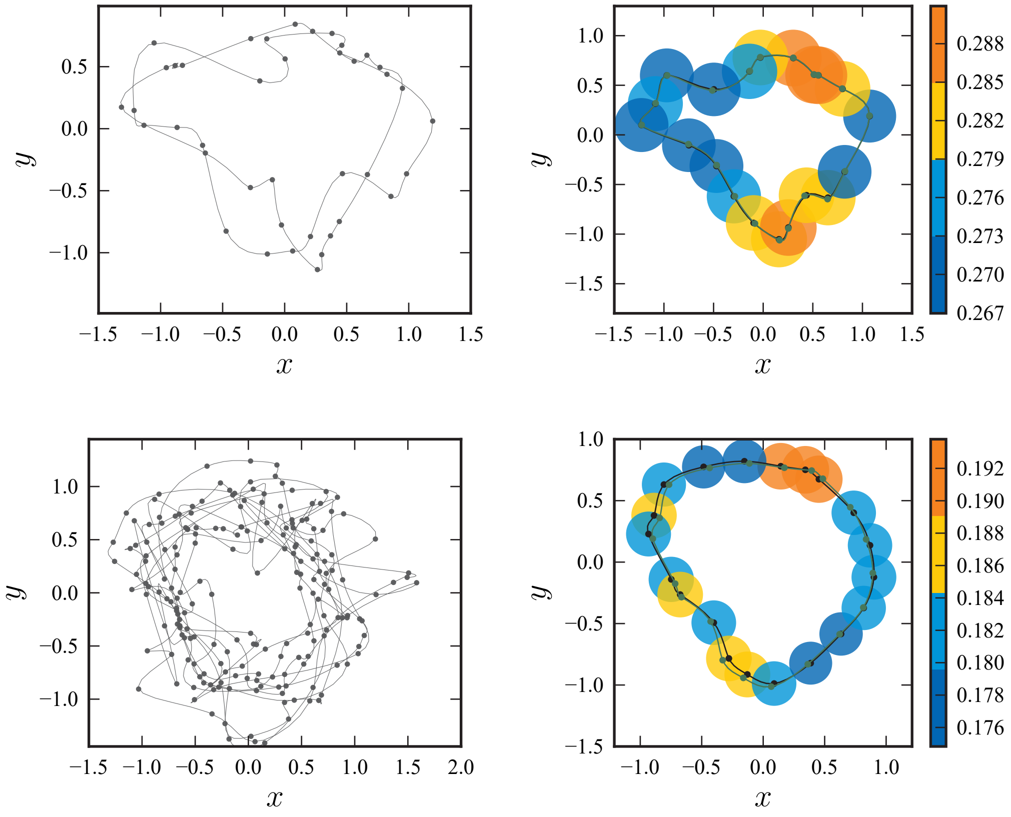

**Figure SM17.** *Second splitting prior. The left-hand plot shows landmark sets and the right-hand plots show averages with green showing the arithmetic average and back showing the MAP point, with one-standard deviation. Here* $\beta = 20$, $\lambda = 0.1$, $\delta^2 = 0.05$.

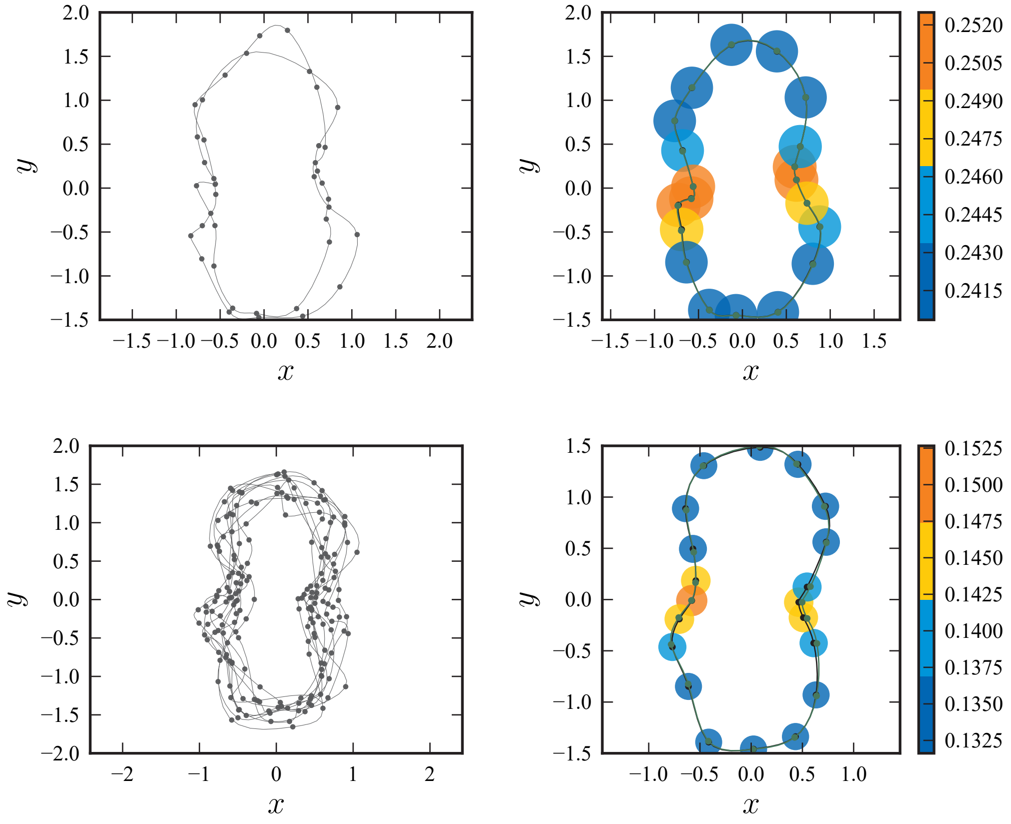


**Figure SM18.** *Second splitting prior. The left-hand plot shows landmark sets and the right-hand plots show averages with green showing the arithmetic average and back showing the MAP point, with one-standard deviation. Here* $\beta = 50$, $\lambda = 0.1$, $\delta^2 = 0.05$.

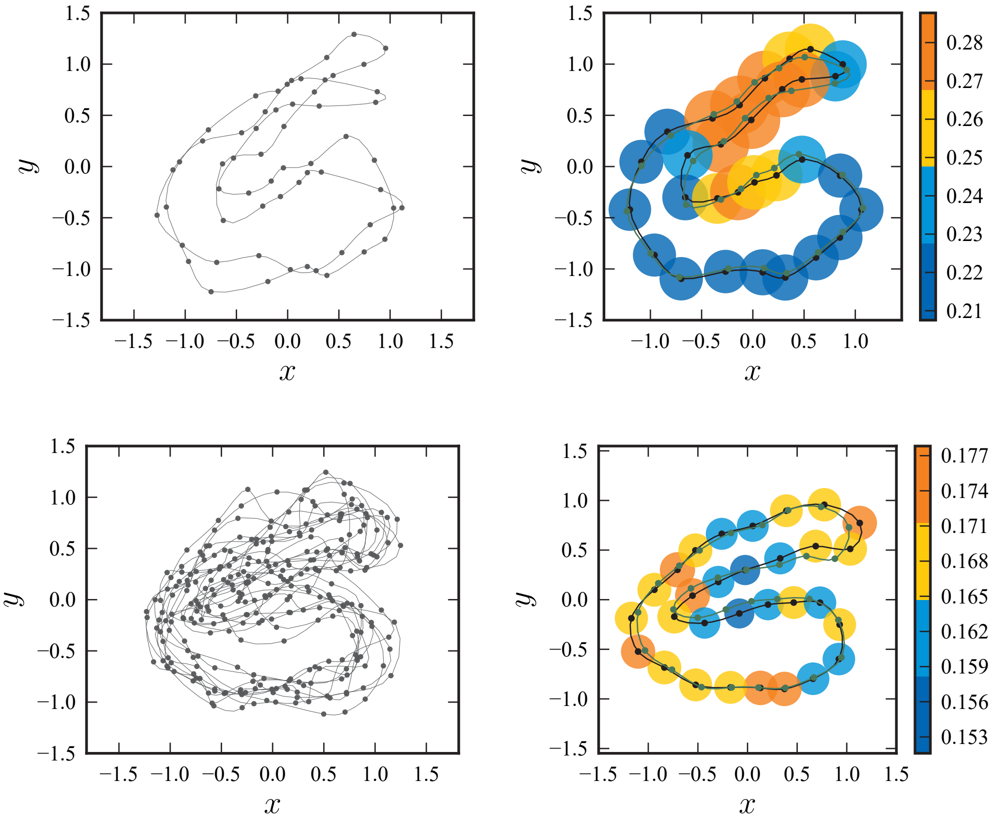


**Figure SM19.** *Second splitting prior. The left-hand plot shows landmark sets and the right-hand plots show averages with green showing the arithmetic average and back showing the MAP point, with one-standard deviation. Here* $\beta = 40$*,* $\lambda = 0.1$*,* $\delta^2 = 0.05$*.*

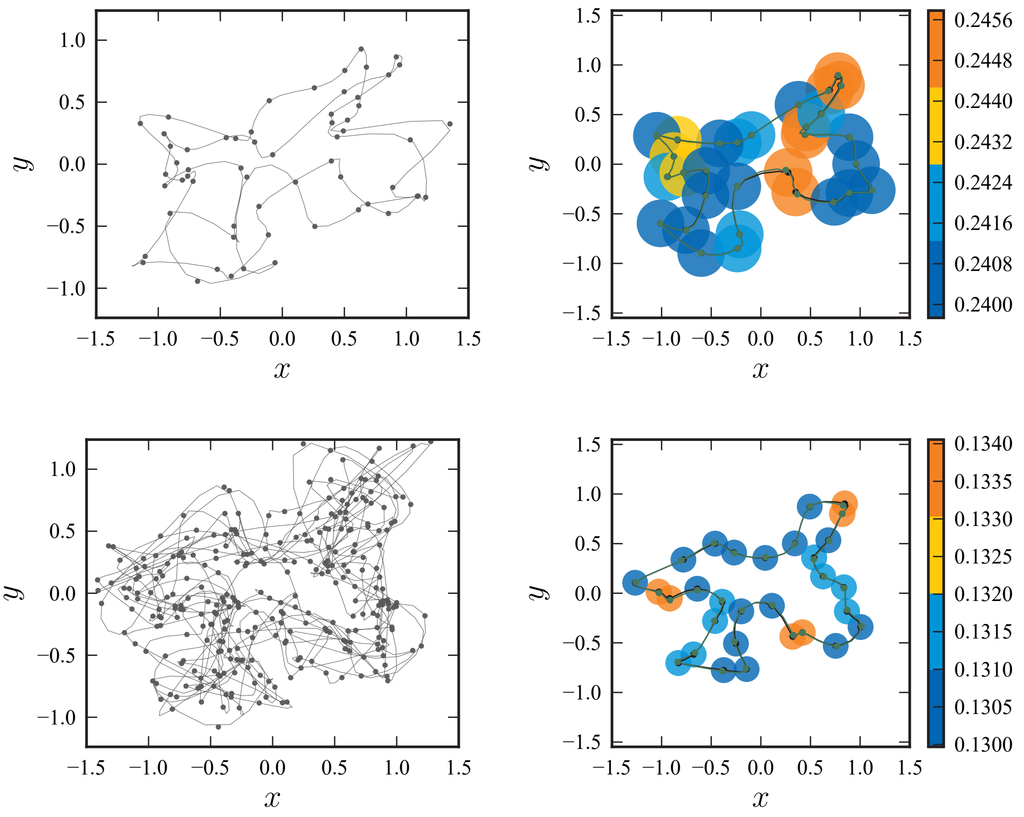


**Figure SM20.** *Second splitting prior. The left-hand plot shows landmark sets and the right-hand plots show averages with green showing the arithmetic average and back showing the MAP point, with one-standard deviation. Here $\beta = 50$, $\lambda = 0.1$, $\delta^2 = 0.05$.*
